# Supplementary material for: Introducing and Interfacing with Cybersecurity -- A Cards Approach
Source: arXiv:2307.16535 source file (2023-07-31)
Supplement: Supplementary file 1 [file appendix_glossary.tex]

% Use one >{\centering\arraybackslash}p{\thin{}} for each option (Strongly disagree, ... Strongly agree).
%\onecolumn
\section{Version 2 Glossary}
\label{app:glossary}

\includegraphics[scale=0.85]{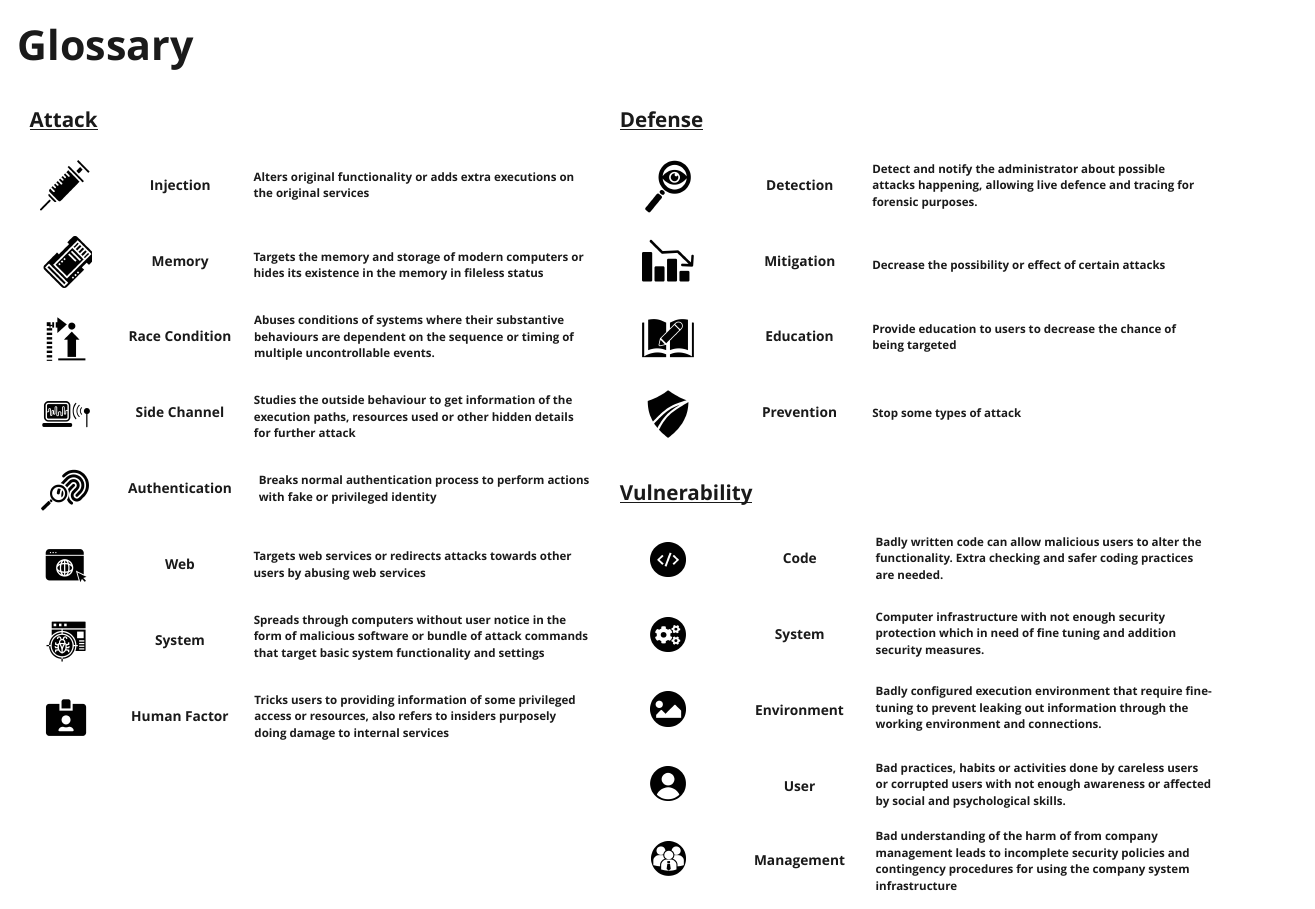}
% \includepdf{glossary.pdf}

%\twocolumn
